# Supplementary material for: Temporal-aware Language Representation Learning From Crowdsourced Labels
Source: arXiv:2107.07958 source file (2021-07-15)
Supplement: Supplementary file 1 [file appendix.tex]

% \section{Robustness to Irresponsible Workers}

% Performance on synthetic data sets are shown in Table \ref{tab:syn_performance}.

% \begin{table*}[!hbpt]
% 	\setlength \tabcolsep{3pt}
% 	\centering
% 	\small
% 	\caption{\label{tab:syn_performance}Accuracy and AUC scores on synthetic data sets.}
% 	\resizebox{0.96\textwidth}{!}{\begin{tabular}{lllllllll}
% 		\toprule
% 		& \multicolumn{2}{c}{2} & \multicolumn{2}{c}{4} & \multicolumn{2}{c}{6} & \multicolumn{2}{c}{8} \\
% 		\cmidrule(lr){2-3} \cmidrule(lr){4-5} \cmidrule(lr){6-7} \cmidrule(lr){8-9}
% 		\# of irresponsible labelers    & \multicolumn{1}{c}{ACC} & \multicolumn{1}{c}{AUC} & \multicolumn{1}{c}{ACC} & \multicolumn{1}{c}{AUC} & \multicolumn{1}{c}{ACC} & \multicolumn{1}{c}{AUC} & \multicolumn{1}{c}{ACC} & \multicolumn{1}{c}{AUC} \\
% 		\midrule
% 		EM                       & 0.876±0.010          & 0.941±0.005          & 0.876±0.010          & 0.941±0.005          & 0.876±0.010          & 0.941±0.005          & 0.876±0.010          & 0.941±0.005          \\
% 		EBCC                     & 0.876±0.013          & 0.942±0.010          & 0.876±0.013          & 0.942±0.010          & 0.876±0.013          & \textbf{0.942±0.010} & 0.876±0.013          & 0.942±0.010          \\
% 		Spectral-EM              & 0.876±0.009          & 0.941±0.004          & 0.876±0.009          & 0.941±0.004          & 0.876±0.009          & 0.941±0.004          & 0.876±0.009          & 0.941±0.004          \\
% 		GLAD                     & 0.878±0.009          & 0.942±0.004          & 0.878±0.009          & 0.942±0.004          & 0.878±0.009          & \textbf{0.942±0.004} & 0.878±0.009          & 0.942±0.004          \\
% 		IBCC                     & 0.876±0.009          & 0.941±0.004          & 0.876±0.009          & 0.941±0.004          & 0.876±0.009          & 0.941±0.004          & 0.876±0.009          & 0.941±0.004          \\
% 		BWA                      & 0.876±0.009          & 0.940±0.004          & 0.877±0.009          & 0.941±0.004          & 0.878±0.009          & 0.941±0.004          & 0.877±0.008          & 0.941±0.004          \\
% 		VI-BP                    & 0.878±0.009          & 0.942±0.004          & 0.878±0.009          & 0.942±0.004          & 0.878±0.009          & \textbf{0.942±0.004} & 0.878±0.009          & 0.942±0.004          \\
% 		VI-MF                    & 0.876±0.009          & 0.941±0.004          & 0.876±0.009          & 0.941±0.004          & 0.876±0.009          & 0.941±0.004          & 0.876±0.009          & 0.941±0.004          \\
% 		KOS                      & 0.878±0.009          & 0.942±0.004          & 0.878±0.009          & 0.942±0.004          & 0.878±0.009          & \textbf{0.942±0.004} & 0.878±0.009          & 0.942±0.004          \\
% 		ZenCrowd                 & 0.876±0.010          & 0.941±0.005          & 0.876±0.010          & 0.941±0.005          & 0.876±0.010          & 0.941±0.005          & 0.876±0.010          & 0.941±0.005          \\
% 		LFC                      & 0.876±0.010          & 0.941±0.005          & 0.876±0.010          & 0.941±0.005          & 0.876±0.010          & 0.941±0.005          & 0.876±0.010          & 0.941±0.005          \\
% 		PM                       & 0.876±0.010          & 0.941±0.005          & 0.876±0.010          & 0.941±0.005          & 0.876±0.010          & 0.941±0.005          & 0.876±0.010          & 0.941±0.005          \\
% 		\midrule
% 		Triple                   & 0.885±0.001          & 0.937±0.001          & 0.880±0.003          & 0.931±0.002          & 0.876±0.010          & 0.928±0.007          & 0.867±0.011          & 0.924±0.008          \\
% 		Centered                 & 0.836±0.005          & 0.901±0.006          & 0.829±0.007          & 0.897±0.005          & 0.825±0.006          & 0.887±0.006          & 0.820±0.008          & 0.884±0.006          \\
% 		RLL-MLE                  & 0.839±0.007          & 0.900±0.002          & 0.849±0.003          & 0.910±0.003          & 0.851±0.005          & 0.903±0.006          & 0.841±0.008          & 0.897±0.009          \\
% 		RLL-Bayesian             & 0.856±0.000          & 0.922±0.002          & 0.847±0.001          & 0.911±0.002          & 0.832±0.000          & 0.897±0.001          & 0.836±0.000          & 0.895±0.001          \\
% 		RECLE                    & 0.839±0.002          & 0.901±0.001          & 0.849±0.009          & 0.919±0.007          & 0.839±0.010          & 0.908±0.012          & 0.822±0.008          & 0.939±0.005          \\
% 		\midrule
% 		LC                       & 0.713±0.010          & 0.719±0.007          & 0.707±0.022          & 0.704±0.013          & 0.706±0.004          & 0.702±0.007          & 0.704±0.023          & 0.710±0.007          \\
% 		DivideMix                & 0.735±0.011          & 0.720±0.015          & 0.727±0.016          & 0.710±0.018          & 0.722±0.011          & 0.710±0.009          & 0.719±0.012          & 0.715±0.018          \\
% 		CrowdLayer               & 0.845±0.010          & 0.906±0.001          & 0.841±0.014          & 0.903±0.001          & 0.842±0.004          & 0.900±0.002          & 0.838±0.006          & 0.899±0.002          \\
% 		\midrule
% 		Triple+EBCC              & 0.888±0.001          & 0.942±0.000          & 0.890±0.002          & 0.941±0.003          & 0.888±0.004          & 0.940±0.006          & 0.889±0.003          & 0.938±0.005          \\
% 		Centered+EBCC            & 0.840±0.005          & 0.907±0.008          & 0.843±0.004          & 0.905±0.003          & 0.841±0.005          & 0.908±0.006          & 0.842±0.004          & 0.910±0.002          \\
% 		LC+EBCC                  & 0.754±0.002          & 0.831±0.006          & 0.754±0.003          & 0.833±0.007          & 0.757±0.005          & 0.827±0.006          & 0.755±0.002          & 0.829±0.008          \\
% 		DivideMix+EBCC           & 0.757±0.008          & 0.832±0.017          & 0.760±0.008          & 0.831±0.011          & 0.761±0.015          & 0.830±0.006          & 0.761±0.011          & 0.831±0.013          \\
% 		\midrule
% 		TACMA                    & \textbf{0.894±0.001} & \textbf{0.946±0.001} & \textbf{0.892±0.002} & \textbf{0.943±0.003} & \textbf{0.896±0.002} & 0.941±0.002          & \textbf{0.893±0.002} & \textbf{0.945±0.003}\\
% 		\bottomrule
% 	\end{tabular}}
% \end{table*}


% \section{Effect of Working Memory Size}

% Effect of different short-term working memory sizes are shown in Table \ref{tab:memory_size}.


% \begin{table*}[!hbpt]
% 	\setlength \tabcolsep{3pt}
% 	\centering
% 	\small
% 	\caption{\label{tab:memory_size} Prediction accuracy and AUC scores with different working memory sizes on 4 real-world data sets.}
% 	\begin{tabular}{cllllllll}
% 		\toprule
% 		& \multicolumn{2}{c}{Commending} & \multicolumn{2}{c}{Emotion} & \multicolumn{2}{c}{Question} & \multicolumn{2}{c}{Concluding} \\
% 		\cmidrule(lr){2-3} \cmidrule(lr){4-5} \cmidrule(lr){6-7} \cmidrule(lr){8-9}
% 		window size	       & \multicolumn{1}{c}{ACC} & \multicolumn{1}{c}{AUC} & \multicolumn{1}{c}{ACC} & \multicolumn{1}{c}{AUC} & \multicolumn{1}{c}{ACC} & \multicolumn{1}{c}{AUC} & \multicolumn{1}{c}{ACC} & \multicolumn{1}{c}{AUC} \\
% 		\midrule
% 		3                    & 0.798±0.009          & 0.862±0.005          & 0.774±0.011          & 0.913±0.022          & 0.853±0.025          & 0.910±0.007          & 0.727±0.008          & 0.828±0.013          \\
% 		4                    & 0.803±0.014          & 0.868±0.004          & 0.781±0.012          & 0.920±0.017          & 0.865±0.022          & 0.924±0.014          & 0.734±0.010          & 0.829±0.012          \\
% 		5                    & 0.800±0.006          & 0.865±0.003          & 0.822±0.008          & 0.938±0.011          & 0.872±0.005          & 0.933±0.004          & 0.749±0.011          & 0.835±0.011          \\
% 		6                    & 0.816±0.008          & 0.870±0.009          & 0.857±0.009          & 0.948±0.006          & 0.873±0.006          & 0.938±0.002          & 0.751±0.012          & 0.840±0.009          \\
% 		7                    & 0.820±0.004          & 0.871±0.006          & 0.889±0.003          & 0.959±0.001          & 0.892±0.008          & 0.936±0.005          & 0.750±0.012          & 0.838±0.010          \\
% 		8                    & 0.828±0.003          & \textbf{0.878±0.005} & \textbf{0.899±0.004} & 0.962±0.003          & 0.897±0.006          & \textbf{0.944±0.004} & \textbf{0.763±0.007} & 0.848±0.014          \\
% 		9                    & \textbf{0.829±0.002} & 0.877±0.005          & 0.895±0.005          & \textbf{0.969±0.003} & \textbf{0.898±0.003} & 0.943±0.003          & 0.762±0.005          & \textbf{0.850±0.011} \\
% 		10                   & 0.825±0.003          & 0.874±0.004          & 0.896±0.004          & 0.967±0.004          & 0.896±0.004          & 0.940±0.003          & 0.761±0.004          & 0.849±0.007          \\
% 		11                   & 0.826±0.002          & 0.875±0.005          & 0.897±0.005          & 0.964±0.005          & \textbf{0.898±0.002} & 0.943±0.004          & 0.762±0.006          & 0.845±0.013       \\
% 		\bottomrule
% 	\end{tabular}
% \end{table*}
